# Supplementary material for: ARGUS: Visualization of AI-Assisted Task Guidance in AR
Source: arXiv:2308.06246 source file (2023-08-11)
Supplement: Supplementary file 1 [file 08-appendix.tex]

\section{Task Examples}
\label{sec:appendix}

\subsection{Cooking scenario / Recipes }

% \myparagraph{Pinwheels}
\subsubsection{Pinwheels}

Ingredients
\begin{itemize}
\item 1 8-inch flour tortilla
\item Jar of nut butter or allergy-friendly alternative (such as sunbutter, soy butter, or seed butter)
\item Jar of jelly, jam, or fruit preserves
\end{itemize}

Tools and Utensils
\begin{itemize}
\item cutting board
\item butter knife
\item paper towel
\item toothpicks
\item ~12-inch strand of dental floss plate
\end{itemize}

Steps
\begin{enumerate}
\item Place tortilla on cutting board.
  \item Use a butter knife to scoop nut butter from the jar. Spread nut butter onto tortilla, leaving 1/2-inch uncovered at the edges.
\item Clean the knife by wiping with a paper towel.
\item Use the knife to scoop jelly from the jar. Spread jelly over the nut butter.
\item Clean the knife by wiping with a paper towel.
\item Roll the tortilla from one end to the other into a log shape, about 1.5 inches thick. Roll it tight enough to prevent gaps, but not so tight that the filling leaks.
\item Secure the rolled tortilla by inserting 5 toothpicks about 1 inch apart.
\item Trim the ends of the tortilla roll with the butter knife, leaving 1⁄2 inch margin between the last toothpick and the end of the roll. Discard ends.
\item Slide floss under the tortilla, perpendicular to the length of the roll. Place the floss halfway between two toothpicks.
\item Cross the two ends of the floss over the top of the tortilla roll. Holding one end of the floss in each hand, pull the floss ends in opposite directions to slice.
\item Continue slicing with floss to create 5 pinwheels.
\item Place the pinwheels on a plate.
\end{enumerate}

\subsubsection{Pour-over Coffee}

Ingredients
\begin{itemize}
\item 12 oz water
\item 25 grams whole coffee beans
\end{itemize}

Tools and Utensils
\begin{itemize}
\item 2-cup liquid measuring cup electric kettle
\item kitchen scale
\item coffee grinder
\item filter cone dripper (stainless steel)
\item paper basket filter (standard 8-12 cup size) 12-ounce coffee mug
\item thermometer
\end{itemize}

Steps
\begin{enumerate}
\item Measure 12 ounces of cold water and transfer to a kettle.
\item Assemble the filter cone. Place the dripper on top of a coffee mug.
\item Prepare the filter insert by folding the paper filter in half to create a semi-circle, and in half again to create a quarter-circle. Place the paper filter in the dripper and spread open to create a cone.
\item Weigh the coffee beans and grind until the coffee grounds are the consistency of coarse sand, about 20 seconds. Transfer the grounds to the filter cone.
\item Check the temperature of the water.
\item Pour a small amount of water in the filter to wet the grounds. Wait about 30 seconds.
\item Slowly pour the rest of the water over the grounds in a circular motion. Do not overfill beyond the top of the paper filter.
\item Let the coffee drain completely into the mug before removing the dripper. Discard the paper filter and coffee grounds.
\end{enumerate}

\subsection{Healthcare and medicine}

\subsubsection{Tourniquet}

Tools
\begin{itemize}
\item Tourniquet
\item Tourniquet label
\item Velcro strap
\item Windlass
\end{itemize}

Steps
\begin{enumerate}
\item Place tourniquet over affected extremity 2-3 inches above wound site.
\item Pull tourniquet tight.
\item Apply strap to strap body.
\item Turn windless clock wise or counter clockwise until hemorrhage is controlled.
\item Lock windless into the windless keeper.
\item Pull remaining strap over the windless keeper.
\item Secure strap and windless keeper with keeper securing device.
\item Mark time on securing device strap with permanent marker.
\end{enumerate}
